# Supplementary material for: Gaussian Splatting Visual MPC for Granular Media Manipulation
Source: arXiv:2410.09740 source file (2025-03-07)
Supplement: Supplementary file 1 [file appendix.tex]

\section*{APPENDIX}

\subsection{Simulated Dataset}
For the simulation experiments, we utilize the environmental setup from Ravens~\cite{corl20_transportnet}. Each task is executed over 100 trials to calculate success rates and state performance. We set up 8 cameras for data collection. To generate the manipulation trajectories, we utilize the oracle policy provided in Ravens\footnote{https://github.com/google-research/ravens}. There are a total 1000 trajectories included in this dataset. The dataset will be released after the paper's acceptance. Through the experiments, we generally have 50 particles in the simulation environment.

\subsection{Gaussian Splatting Reconstruction}
\label{app:gs_recon}
For Gaussian splatting reconstruction, we follow the implementation provided in \href{https://github.com/graphdeco-inria/gaussian-splatting}{this repository}. The framework is optimized using the Adam optimizer~\cite{adam} with a learning rate of 0.001 over 2000 epochs. The loss function used for training Gaussian splatting is:
\begin{equation}
\mathcal{L} = \mathcal{L}_{L1} + 0.25 \cdot (1 - \mathcal{L}_{SSIM})
\end{equation}
, where $\mathcal{L}_{L1}$ and $\mathcal{L}_{SSIM}$ are L1 loss and structure similarity metrics between the reconstructed image and ground-truth image.

\subsection{Dynamic Model Training}
\label{app:dyna}

Our dynamic model $f$ consists of three components: $f_{enc}$, $f_{mp}$, and $f_{dec}$. The encoder, $f_{enc}$, is composed of two SAGE layers~\cite{neurips17_sage} with a hidden dimension of 256 and ReLU activation functions. The message-passing module, $f_{mp}$, includes two SAGE layers with two recursive message-passing steps. The decoder, $f_{dec}$, is composed of a single SAGE layer. The dynamic model is optimized using the Adam optimizer~\cite{adam} with a learning rate of 0.001, without applying any learning rate scheduler.

For the graph forming part, the distance threshold $\omega$ used was 0.1.

\subsection{Baseline Implementation}
In this section, we provide implementation details for each baseline.

\textbf{Dynamic resolution}~\cite{rss23_dyna_resolution}.
We adapt the official implementation from \href{https://RoboPIL.github.io/dyn-res-pile-manip/}{this link}. To ensure a fair comparison, we convert our dataset into their format and use the hyperparameters provided by the authors in the appendix.

\textbf{NeRF-dy}~\cite{corl21_nerfdy}.
We implemented this approach using the source code provided by the authors. To maintain fairness, we converted our dataset into their format and applied the hyperparameters provided in their appendix.

\textbf{NFD}~\cite{corl23_neural_field}.
Since the official implementation is not available, we re-implemented this method based on the hyperparameters and network architecture described in the paper and supplementary materials. We verified the validity of our implementation by comparing its performance to the results reported in \cite{corl23_neural_field}.

\textbf{DVF}~\cite{wafr20_}.
Since the official implementation is not available, we re-implemented this method based on the hyperparameters and network architecture described in the paper and supplementary materials. We verified the validity of our implementation by comparing its performance to the results reported in \cite{wafr20_}.

\subsection{Real-World Experiments}
Franka Panda manipulator and four Intel RealSense
D415. Each task is executed over 20 trials to calculate success rates. 

\newpage
